# Supplementary material for: Executable Refinement Types
Source: arXiv:1403.3336 source file (2014-03-13)
Supplement: Supplementary file 1 [file appendix.tex]

\clearpage
\section{Type Soundness}
(including proofs of claims from from subsection~\ref{subsec:type:correct})

\pfshortnumbers{5}

\subsection{Weakening}

\begin{lemma}
  \label{lemma:weakening}
  Let 
  \(
  \begin{array}[t]{rcl}
    E  & = & E_1,E_2 \\
    E' & = & E_1,x:U,E_2
  \end{array}
  \)
  
  \begin{enumerate}
  \item
    If $\judgeT{E}{T}$ and $\judgeT{E}{S}$ then if
    $\judgesub{E}{S}{T}$ then $\judgesub{E'}{S}{T}$.
  \item
    If $\judge{E}{t}{T}$ then $\judge{E'}{t}{T}$.
  \item
    If $\judgeT{E}{T}$ then $\judgeT{E'}{T}$.
  \end{enumerate}
\end{lemma}

\proof\

\begin{list}{}{}
\item{(1)} By straightforward induction on the derviation of
  $\judgesub E S T$, using the Weakening axiom of theorem proving in
  the base case for rule \rel{S-Base}

\item{(4) and (5)} By straightforward mutual induction on the
  derivations of $\judge E t T$ and $\judgeT E T$, using part $(1)$ in
  the case of rule \rel{T-Sub}
  \qed
\end{list}

\subsection{Substitution}

\begin{lemma}[(Substitution)]
  \label{lemma:substitution}
  Suppose
  \[
  \begin{array}{l}
    \judge{E_1}{s}{S} \\
    \theta = \subst x s S \\
    E=E_1,x:S,E_2\\
    E'=E_1,\theta E_2
  \end{array}
  \]
  Then:
  \begin{enumerate}
  \item If $\judgesub{E}{T_1}{T_2}$ then $\judgesub{E'}{\theta T_1}{\theta T_2}$.
  \item If $\judgeT{E}{T}$ then $\judgeT{E'}{\theta T}$.
  \item If $\judge{E}{t}{T}$ then $\judge{E'}{\theta t}{\theta T}$ 
    % and $\judgesub{E'}{T'}{\theta T}$.
  \end{enumerate}
\end{lemma}

\proof\

\begin{list}{}{}
\item{(1)} By straightforward induction on the derivation $\judgesub E {T_1} {T_2}$
  using the Substitution axiom of theorem proving.
\item{(2) and (3)} By straightforward mutual induction on the derviations
  $\judge E t T$ and $\judgeT E T$.  The case for \rel{T-Sub} uses
  part $(1)$, and in the case for \rel{T-Var} if $t = x$ then $S = T$ and
  $\theta t = s$ and we use weakening to extend
  $\judge {E_1} s S$ to $\judge {E'} s S$.\qed
\end{list}

\subsection{Properties of Subtyping}

\begin{lemma}[(Narrowing of Subtyping)]\
  \label{lemma:NarrowingOfSubtyping}

  If $\judgesub E S T$ and $\judgesub {E,x:T,F} Q R$ then $\judgesub
  {E,x:S,F} Q R$.
\end{lemma}

\proof\ By straightforward induction over the derivation of $\judgesub
{E,x:T,F} Q R$ using the Narrowing axiom of implication.\qed

\begin{lemma}[(Subtyping is a Preorder-in-context)]\
  \label{lemma:SubtypingPreorder}

  \begin{enumerate}
  \item If $\judgeT E T$ then $\judgesub E T T$
  \item If $\judgesub E S T$ and $\judgesub E T U$ then $\judgesub E S U$
  \end{enumerate}
\end{lemma}

\proof\

\begin{enumerate}
\item By induction on the derivation of $\judgeT E T$, using the
  Reflexivity axiom of theorem proving.
\item By induction on the derivation of $\judgesub E S T$ (followed by
  inversion on $\judgesub E T U$) using Lemma
  \ref{lemma:NarrowingOfSubtyping} (Narrowing of Subtyping) for the
  bindings in function types, and the Transitivity axiom of theorem
  proving. \qed
\end{enumerate}

\subsection{Preservation}

In the following, we lift the notation $S \lred T$ for evaluation
of an arbitrary subterm of $S$, yielding $T$.

\begin{lemma}[(Type Equivalence under Evaluation)]
  If $\judgeT E S$ and $S \lred T$ then $\judgesubsub E S T$.
  \label{lemma:TypeEval}
\end{lemma}

\proof\ By induction on the derivation of $S$.  In
the base case of \rel{WT-Base} we invoke the Evaluation axiom of theorem
proving.\qed

\restatepreservation

\begin{lamproof}
  \pf\ By induction on the typing derivation $\judge{E}{s}{T}$, with case analysis
  on the final rule applied.
  
  \proofcase\ \rel{T-Var}, \rel{T-Const}: No evaluation rule applies.

  \proofcase\ \rel{T-Cast}: By Lemma \ref{lemma:TypeEval} (Type
  Equivalence under Evaluation) evaluating either of the types in a
  cast does not change its type.
  
  \proofcase\ \rel{T-Fun}, \rel{T-Sub}: Immediate from the inductive hypothesis
  and Lemma \ref{lemma:TypeEval}.
    
  \rulecase{T-Checking}
  \begin{lamproof}
    \proofcase\ $\checkingpred x B t s c \lred \checkingpred x B t {s'} c$
    \qpf{Apply \rel{T-Checking} using the Evaluation property of implication}
    
    \proofcase\ $\checkingpred x B t s c \lred \checkingpred x B {t'} s c$
    \qpf{By Lemma \ref{lemma:TypeEval} the type is equivalent so apply
      \rel{T-Checking} and then \rel{T-Sub}
    }
    
    \proofcase{$\checkingpred x B t \true c \lred c$}
    \qpf{
      By assumption, $c$ has singleton type
      $\predty x B {x = c}$ and since
      we know \true implies $\subst x c B\, t$,
      by the Hypothesis property of implication,
      $\judgeimp {x:B} {x=c} {t}$ so we can assign
      $\predty x B t$ to $c$.
    }
  \end{lamproof} % T-Checking
  
  \rulecase{T-App} Consider the possible evaluation rules:
  \begin{lamproof} 
    
    \rulecase{E-Prim}: Preservation holds by assumption 1 on constants.
    
    \rulecase{E-$\beta$}: Apply Lemma \ref{lemma:substitution} (Substitution)
  
    \rulecase{E-Compat}: Apply the inductive hypothesis and in
    Lemma \ref{lemma:TypeEval} (Type equivalence under evaluation).
    
    \rulecase{E-Cast-Begin}: Then a constant $c$ of some refinement of $B$ is being
    cast to some well-formed $\predty x B t$.  Using reflexivity of theorem
    proving, we derive:\\\
    
    \(
    \Concluderule {\rel{T-Checking}} {
      \judge E {\checkingpred x B t {\subst x c B \, t} c} {\predty x B t}
    } {
      \judgeT E {\predty x B t}
      \and
      \judge E c B
      \and
      \judgeimp E {\subst x c B\, t} {\subst x c B\, t}
    }
    \)
    \\\
  
    \rulecase{E-Cast-F}: A term $f$ of type $(\lamt x {S_1} {S_2})$ is
    being cast to the well-formed type $(\lamt x {T_1} {T_2})$.  We thus
    derive:\\\
  
    \(
    \Concluderule{T-Fun}{
      \judge E {\funcastltwo {} x {S_1} {S_2} f {T_1} {T_2}} {\lamt x {T_1} {T_2}}
    } {
      \vdots
    }
    \)
  \end{lamproof} % T-App
  \qed
\end{lamproof} % Preservation

\subsection{Progress}

\begin{lemma}[(Canonical Forms)]
  If $\judge{}{v}{(\lamt{x}{T_1}{T_2})}$ then either
  \begin{enumerate}
  \item $v=\lam{x}{S}{s}$ and $\judgesub{}{T_1}{S}$ and $\judge{x:S}{s}{T_2}$, or
  \item $v$ is a constant and $\fun{ty}(c)$ is a subtype of $\lamt{x}{T_1}{T_2}$.
  \item $v$ is a cast $\cast {S_1} {S_2}$ where $\judgesub {} {T_1} {S_1}$
    and $\judgesub {} {S_2} {T_2}$.
  \end{enumerate}
\end{lemma}

\begin{lamproof}
  \pf\ By induction on $\judge{}{v}{\lamt x {T_1} {T_2}}$.
  
  \rulecase{T-Var} Does not apply to values

  \rulecase{T-Const} Then we are in case 2.

  \rulecase{T-Fun} Then $v = \lam x {T_1} s$ and $\judge {x:S} s {T_2}$ so
  by reflexivity of subtyping we meet case 1.

  \rulecase{T-Cast} Then $v = \cast {T_1} {T_2}$ and by reflexivity of subtyping
  we are in case 3.

  \rulecase{T-Checking} Cannot apply to values

  \rulecase{T-Sub} The lemma follows by induction and transitivity of subtyping.
  \qed
\end{lamproof}

\StateProgress

\proof\ By induction on the derivation of $\judge E t T$.
\begin{lamproof}
  \proofcase\ \rel{T-Var}, \rel{T-Const}, \rel{T-Fun}, \rel{T-Cast}: Then $t$ is already a value.

  \proofcase\ \rel{T-Sub}: Immediate from the inductive hypothesis.
  
  \rulecase{T-App}: Then $t = t_1 ~ t_2$.  If $t_1$ or $t_2$ are not values, then by
  induction they can evaluate hence $t$ can as well.  If both are values, then there are three possible forms for $t_1$
  (given by Canonical forms):
  \begin{enumerate}
  \item $t_1$ is a constant of appropriate type - then its meaning
    function can be applied.
  \item $t_1$ is a lambda term, so $\beta$-reduction applies.
  \item $t_1$ is a cast.  If $t_1$ is a cast to a base type, then
    canonical forms tells us that $t_2$ is a constant so
    \rel{E-Cast-Begin} applies.  Otherwise, $t_1$ is a function cast
    so \rel{E-Cast-F} applies.
  \end{enumerate}

  \rulecase{T-Checking}: Then we have $t = \checkingpred x B p s c$, where\\\

    \(
    \Concluderule {\rel{T-Checking}} {
      \judge {} {\checkingpred x B p s c} {\predty x B p}
    } {
      \judgeT {} {\predty x B t}
      \and
      \judge {} c B
      \and
      \judgeimp {} s {\subst x c B\, p}
    }
    \)
    \\\

    If $s$ is not a value, then by induction $s$ can evaluate
    or is a failed cast (hence this cast is failed too).
    If $s = \true$, then we
    can evaluate by \rel{E-Cast-End}.  If $s = \false$ then by
    definition this is a failed cast.
\end{lamproof}

\clearpage
\section{Correctness of Hybrid Type Checking}
(Including proofs of claims in Section~\ref{subsec:bisim})

\subsection{Preliminary Lemmas}

% Now built in
% \begin{lemma}[(Transitivity of Similarity)]
%  \begin{enumerate}
%  \item If $\judgesimt E s t S$ and $\judgesimt E t u T$ then
%    $\judgesimt E s u S$
%  \item If $\judgesimty E S T$ and $\judgesimty E T U$ then
%    $\judgesimty E S U$
%  \end{enumerate}
%\end{lemma}
%
%\proof\ By mutual induction on the derivations.

%\begin{lemma}[(Bisimilar Substitution Into Identical Contexts)]
%  \label{lemma:BisimSubstSimple}
%  Suppose $\judgesimt E {s_1} {s_2} S$, then let
%  $\theta_1 = \subst x {s_2} S$ and $\theta_2 = \subst x {s_2} S$
%
%  \begin{enumerate}
%  \item If $\judge {E, x:S, F} t T$ 
%    then $\judgesimt {E,\theta_* F} {\theta_1 t} {\theta_2 t} {\theta_* T}$
%  \item If $\judgeT {E, x:S, F} T$ then
%    $\judgesimty {E, \theta_* F} {\theta_1 T} {\theta_2 T}$
%  \end{enumerate}
%\end{lemma}

%\begin{lamproof}
%  \proof\ By mutual induction on the derivations of $\judge {E, x:S, F} t T$ 
%  and $\judgeT {E, x:S, F} T$.
%
%  \rulecase{\rel{T-Sub}}: By induction
%
%\end{lamproof}

\begin{lemma}[(Bisimilarity is reflexive)]
  \label{lemma:bisimreflexive}
  If $\judge E t T$ then $\judgesimt E t t T$
\end{lemma}

\pf\ By induction on the typing derivation. \qed

\begin{lemma}[(Bisimilar Substitution)]
  \label{lemma:bisimsubst}
  Suppose $\judgesimt E {s_1} {s_2} S$, then let
  $\theta_1 = \subst x {s_2} S$ and $\theta_2 = \subst x {s_2} S$

  \begin{enumerate}
  \item If $\judgesimt {E, x:S, F} {t_1} {t_2} T$ 
    then $\judgesimt {E,\theta_1 F} {\theta_1 t_1} {\theta_2 t_2} {\theta_1 T}$
  \item If $\judgesimty {E, x:S, F} {T_1} {T_2}$ then
    $\judgesimty {E, \theta_1 F} {\theta_1 T_1} {\theta_2 T_2}$
  \end{enumerate}
\end{lemma}

\begin{lamproof}
  \proof\ By mutual induction on the derivations of 
  $\judgesimt {E,x:S,F} {t_1} {t_2} T$ and $\judgesimty {E,x:S,F} {T_1} {T_2}$

  \rulecase{Eq-Arrow}: Immediate from induction.

  \rulecase{Eq-Base}: Immediate from mutual induction.

  \rulecase{Up-Trans}: 
  By induction $\judgesimt {E,\theta_1 F} {\theta_1 s} {\theta_1 t} {\theta_1 T}$
  (since $s_1$ is similar to itself) and 
  $\judgesimt {E,\theta_1 F} {\theta_1 t} {\theta_2 u} {\theta_1 T}$
  so apply \rel{Up-Trans}.

  \rulecase{Up-Sub}: By induction and Lemma \ref{lemma:substitution} 
  (Substitution) rule \rel{Up-Sub} applies.

  \rulecase{Up-Equiv}: By induction, using Lemma \ref{lemma:upcast:reflexive}
  (Bisimilarity is reflexive) to apply $\theta_1$ to the types.
  
  \rulecase{Up-Const}: Trivial.

  \rulecase{Up-Var}: Identical to Lemma \ref{lemma:substitution} (Substitution)

  \proofcase{\rel{Up-App}, \rel{Up-Fun}, \rel{Up-Cast}}: All follow by
  induction and mutual induction.
  
  \rulecase{Up-Checking}: Induction plus the Substitution property of
  implication.

  \rulecase{Up-Add}: Same as \rel{Up-Sub}

  \rulecase{Up-Eta}: By induction, since new variable must be chosen fresh.
  \mynote{enforce this in the type rules}

  \rulecase{Up-AddChecking}: By induction and the Substitution property
  of implication.\qed

\end{lamproof}

\subsection{Bisimulation}

\newcommand{\bigred}{\Rrightarrow}
Define $\lred_c$ to be reduction
via \rel{E-Cast-F} in any context; this reduction relation characterizes some
``administrative'' reductions that occur in the proof of bisimulation.
Then define $\bigred$ to be $\lred \circ \lred_c^*$, that is any number of
$\lred_c$ reductions followed by exactly one usual reduction.
We prove bisimulation with respect
to this evaluation relation, which contains single step evaluation.

\begin{lemma}[(Function Cast Bisimulation)]
  \label{lemma:fcastbisim}
  Suppose $\judgesimt E s t T$

  \begin{enumerate}
  \item If $s \lred_c s'$ then there is some $t'$ such that
    $t \lred_c t'$ and $\judgesimt E {s'} {t'} T$
  \item If $t \lred_c t'$ then $\judgesimt E s {t'} T$
  \end{enumerate}
\end{lemma}

\begin{lamproof}
  By induction on the derivation of $\judgesim E s t T$.

  \rulecase{Up-Var, Up-Const} No reduction is possible.

  \rulecase{Up-Trans, Up-Fun, Up-Cast, Up-Sub, Up-Checking,Up-Add,Up-Eta} 
  Immediate by induction.

  \rulecase{Up-App} Then $s = s_1~s_2$ and $t = t_1~t_2$.
  If reduction occurs in a subterm, then the conclusion
  is immediate by induction.  Otherwise, $s_1$ and $t_1$ must be
  casts to bisimilar function types, so the results of expansion
  are bisimilar.

  \rulecase{Up-Add} The conclusion is immediate by induction
  except when $t = \casttwoapp {\lamt x {S_1} {S_2}} {\lamt x {T_1} {T_2}} {t_1}$.
  Then $\judgesimt E s {t_1} {\lamt x {S_1} {S_2}}$ so after expansion
  we can apply \rel{Up-Eta} and \rel{Up-Add}. \qed
\end{lamproof}

\begin{coro}
  \label{lemma:fcastbisimplus}
  Suppose $\judgesimt E s t T$

  \begin{enumerate}
  \item If $s \lred_c^+ s'$ then there is some $t'$ such that
    $t \lred_c^+ t'$ and $\judgesimt E {s'} {t'} T$
  \item If $t \lred_c^+ t'$ then $\judgesimt E s {t'} T$
  \end{enumerate}
\end{coro}

\begin{lemma}[(Big-step Function Cast Bisimulation)]
  \label{lemma:fcastbisimvalue}

  Suppose $\judgesimt E s t T$

  \begin{enumerate}
  \item If $s \lred_c^* s'$ where $s'$ is a value then there exists a value $t'$
    such that $t \lred_c^* t'$ and $\judgesimt E {s'} {t'} T$
  \end{enumerate}
\end{lemma}

\begin{lamproof}

  \pf\ By induction on the length of $s \lred^* s'$ followed
  by induction on $\judgesimt E s t T$.
  
  \rulecase{Up-Const, Up-Var, Up-Fun, Up-Cast}  
  Both $s$ and $t$ are already bisimilar values.

  \rulecase{Up-Equiv, Up-Sub, Up-Checking, Up-Eta} Immediate by induction.

  \rulecase{Up-App} Then since $s$ is not already a value,
  $s \lred_c s'' \lred_c^* s'$ and by \ref{lemma:fcastbisim} we acquire
  $t''$ bisimlar to $s''$.  Then by induction on the length of evaluation
  we apply the lemma to the reduction sequence $s'' \lred_c^* s'$.
  
  \rulecase{Up-Trans} Then $\judgesimt E s u T$
  and $\judgesimt E u t T$.  If $u$ is already a value, then the
  conclusion follows by induction on the second subderivation.
  If $u$ is not a value, then by induction on the first subderivation
  we acquire the value $u'$ and by Corollary \ref{lemma:fcastbisimplus}
  we acquire a corresponding $t'$ and then apply \rel{Up-Trans}

  \rulecase{Up-Add} There are two cases for what $t$ could be:
  \begin{lamproof}
    \proofcase{$t = \casttwoapp {\predty x B p} {\predty x B q} {t_1}$}
    Then by canonical forms $s = c$ and
    by induction and canonical forms $t_1$ evaluates to $c$.  Then
    $t$ reduces to a check in progress, which must evaluate to \true\
    by the Evaluation property of theorem proving, hence $t$ evaluates
    to $c$ which is bisimilar by \rel{Up-Const}.

    \proofcase{$t = \casttwoapp {\lamt x {S_1} {S_2}} {\lamt x {T_1} {T_2}} {t_1}$}
    Then after expanding the function cast, $t$ reduces to a value
    bisimilar to $s$.
  \end{lamproof}

  \rulecase{Up-AddChecking} By canonical forms $s' = c$ and
  by the Evaluation and Consistency properties
  of implication, $t$ evaluates to $c$.
  \qed
\end{lamproof}

\begin{lemma}[Augmented Bisimulation]
  Suppose $\judgesimt E s t T$

  \begin{enumerate}
  \item If $s \bigred s'$ then there is some $t'$ such that
    $t \bigred t'$ and $\judgesimt E {s'} {t'} T$
  \item If $t \bigred t'$ then there is some $s'$ such that
    $s \bigred^{0/1} s'$ and $\judgesimt E {s'} {t'} T$
  \end{enumerate}
\end{lemma}

\begin{lamproof}
  \pf\ By induction on the derivation of $\judgesimt E s t T$.

  \rulecase{Up-Const,Up-Var} No evaluation is possible.

  \rulecase{Up-Trans,Up-Sub,Up-Fun,Up-Cast,Up-Checking} Immediate by induction.
  
  \rulecase{Up-Add} Then $t = \casttwoapp S T {t_1}$ where\\\
  
  \[
  \concluderule{\rel{Up-Add}}{
    \judgesim{E}{s}{\casttwoapp S T {t_1}}
  }{
    \judgesimt E s {t_1} S
    \and
    \judgesub E S T
  }
  \]
  
  \begin{lamproof}
    \proofcase{$s \bigred s'$ or $t_1 \bigred t_1'$} Immediate by induction.
    
    \proofcase{
      $t = \casttwoapp {\predty x B p} {\predty x B q} {c} 
      \bigred \checkingpred x B q {\subst x c B\, q} c$
    }
    Then by induction and the Substitution property of theorem proving we can
    apply \rel{Up-AddChecking}.
    
    \proofcase{
      $t = \casttwoapp {\lamt x {S_1} {S_2}} {\lamt x {T_1} {T_2}} {t_1}
      \bigred 
      \funcastltwo {} x {S_1} {S_2} {t_1} {T_1} {T_2}$
    }
    Then by induction $\judgesimt s {t_1} {\lamt x {S_1} {S_2}}$
    so we can apply \rel{Up-Eta} and \rel{Up-Add}.
    
  \end{lamproof}
  
  \rulecase{Up-AddChecking} Then $t = \checkingpred x B q {t_1} c$ 
  and $\judgesimt s c {\predty x B q}$
  and there are two cases to consider.
  \begin{lamproof}
    \proofcase{$t_1 \bigred t_1'$} By the evaluation
    axiom of theorem proving, nothing changes.
    
    \proofcase{$t_1 = \true$} Then $t \bigred c$ and
    $\judgesimt E s c T$ so we are done.
  \end{lamproof}
    
  \rulecase{Up-Eta} Then $t = \lam x S {t_1~x}$.  If $t_1~x \lred t_1'$,
  then since $\judgesimt E s {t_1} {\lamt x S T}$, the argument
  that $s$ can match $t_1$ is a simpler version of the below case for 
  \rel{Up-App}

  \rulecase{Up-App} Assume $t \bigred t'$ since the possible forms
  for $t$ are a superset of those for $s$.  Consider the
  non-administrative reduction step:
    
  \begin{lamproof} 
    
    \rulecase{E-Compat}  Immediate by induction.

    \rulecase{E-Beta}
    Then $t = t_1~t_2 = (\lam x {T_1} {t_b})~t_2 
    \bigred \subst x {t_2} {T_1}\, {t_b}$.
    But $s = s_1~s_2$ where $s_1 \lred_c^* s_1'$ a value bisimilar
    to $t_1$ by Lemma \ref{lemma:fcastbisimvalue}.  We consider
    the possible shapes:

    \begin{lamproof}
      \proofcase{$s_1 = \lam x S {s_b}$}: Then we
      can reduce and by Lemma \ref{lemma:bisimsubst} 
      $\judgesimt E {\subst x {s_2} S\, s_b} {\subst x {t_2} T\, t_b} {\subst x {s_2} S\, T}$.
      
      \proofcase{$s_1 = c$ for some function constant:} Then $t_1$ can
      only be an $\eta$ expansion of $c$ so the reduction just
      collapses this and bisimilarity is immediate.
    \end{lamproof}

    \rulecase{E-Prim} Then $t = c~t_2 \bigred \meaningf{c}(t_2)$ and
    we assume constants respect bisimilarity.

    \rulecase{E-Cast-Begin,E-Cast-F} Then $s$ and $t$ are casts of
    bisimilar values to/from bisimilar types, and they evaluate
    in lock step.
    \qed
  \end{lamproof}
\end{lamproof}

Then, since $\lred$ is a subrelation of $\bigred$, bisimilarity
is immediate.

%\restatebisim

\begin{coro}
  \label{lemma:ctxequiv}
  If $\judgesimt E s t T$ then $s$ and $t$ are contextually equivalent.
\end{coro}

\begin{coro}
  \label{lemma:tyequiv}
  If implication respects contextual equivalence
  and $\judgesimty E S T$ then $\judgesub E S T$ and $\judgesub E T S$
\end{coro}

%===========================================================================

\clearpage
\subsection{Cast Insertion}
\begin{lemma}
\label{lem:sub:bisim}
If $\judgeE{(E,x:U)}$ and $\judgeT{E,x:U}{S}$ and $\judgesub{E,x:U}{S}{T}$ and 
$\judge{E}{s}{U}$ and $\judgesim{E}{s}{t}$ then $\judgesub{E}{S[x:=s]}{T[x:=t]}$.
\end{lemma}
\begin{proof}
By induction on the subtyping derivation.
\end{proof}

\restatecastinsertbisim

\begin{lamproof}
  \pf\ By mutual induction on the cast insertion derivations.  
  \comment{
    Though
    typing is not syntax directed, the case where the typing derivation ends
    with subtyping need not be considered as it can be eliminated by an induction 
    on whether subtyping was the last rule applied.
  }
  
  \rulecase{C-Const} Then $\judgesimt E c c {ty(c)}$ by \rel{Up-Const}

  \rulecase{C-Var} Since $\judgec E x x T$ and $\judge E x S$, 
  hence $\judgesub E T S$ because $S = T$ 
  and $\judgesimt E x x S$ by \rel{Up-Var}
  
  \rulecase{C-Fun} 
  \begin{lamproof}
  In this case: 
  \[
  \begin{array}[t]{l@{\qquad}l}
    \judge{E}{(\lam{x}{S}{s})}{(\lamt{x}{S}{S'})}
    & 
    \judgec{E}{(\lam{x}{S}{s})}{(\lam{x}{T}{t})}{(\lamt{x}{T}{T'})}
    \\
    \judgeT{E}{S}
    &
    \judgect{E}{S}{T} 
    \\
    \judge{E,x:S}{s}{S'}
    &
    \judgec{E,x:T}{s}{t}{T'} 
  \end{array}
  \]

  Then by induction (using narrowing)
  \[
  \begin{array}[t]{l}
    \judgesimty E S T \\
    \judgesimt {E,x:S} s t {S'} \\
    \judgesimty {E,x:S} {S'} {T'}
  \end{array}
  \]

  So by \rel{Eq-Arrow} and \rel{Up-Fun}, respectively
  \[
  \begin{array}[t]{l@{\qquad}l}
    \judgesimty E {\lamt x S {S'}} {\lamt x T {T'}} \\
    \judgesimt E {\plam x S s} {\plam x T t} {\plamt x S {S'}}\\
  \end{array}
  \]
  \end{lamproof} % C-Fun

  \rulecase{C-App}
  \begin{lamproof} % C-App
    In this case
    \[
    \begin{array}[t]{l@{\qquad}l}
      \judge E {s_1 ~ s_2} {\subst x {s_2} {}\, S}
      &
      \judgec E {s_1 ~ s_2}{t_1 ~ t_2} {\subst x {t_2} {}\, T'}
      \\
      \judge{E}{s_1}{(\lamt{x}{S}{S'})}
      & 
      \judgec{E}{s_1}{t_1}{(\lamt{x}{T}{T'})}
      \\
      \judge{E}{s_2}{S}
      & 
      \judgecc{E}{s_2}{t_2}{}{T} 
    \end{array}
    \]

    Then by induction and inversion
    \[
    \begin{array}[t]{l}
      \judgesimt E {s_1} {t_1} {\lamt x S {S'}}\\
      \judgesimty E {\lamt x S {S'}} {\lamt x T {T'}} \\
      \judgesimty E S T \\
      \judgesimty {E,x:S} {S'} {T'} \\
      \judgesimt E {s_2} {t_2} S
    \end{array}
    \]

    Hence by \rel{Up-App} and Lemma \ref{lemma:bisimsubst}, respectively
    \[
    \begin{array}[t]{l}
      \judgesimt E {s_1~s_2} {t_1~t_2} {\subst x {s_2} {}\, S'} \\
      \judgesimty E {\subst x {s_2} {}\, S'} {\subst x {t_2} {}\, T'}
    \end{array}
    \]
  \end{lamproof} % C-App

  \rulecase{C-Cast} Immediate by induction as in above two cases.

  \proofbreak

  \rulecase{CC-Ok}
  \begin{lamproof}
    In this case
    \[
    \begin{array}[t]{l@{\qquad}l}
      \judge E s S & \judgec E s t {S'} \\
      \judgesimty E S T & \judgecc E s t {} T \\
    \end{array}
    \]
    
    By induction
    \[
    \begin{array}[t]{l}
      \judgesimt E s t S \\
      \judgesimty E {S'} S \\
    \end{array}
    \]

    Hence $\judgesimty E {S'} T$ by transitivity
    and 
    $\judgesimt E s t T$
    by \rel{Up-Equiv}

  \end{lamproof}
    
  \rulecase{CC-Ok}
  \begin{lamproof}
    In this case
    \[
    \begin{array}[t]{l@{\qquad}l}
      \judge E s S & \judgec E s t {S'} \\
      \judgesimty E S T & \judgecc E s {\casttwoapp {S'} T t} {} T \\
    \end{array}
    \]

    Then by induction
    \[
    \begin{array}[t]{l}
      \judgesimt E s t S \\
      \judgesimty E {S'} S
    \end{array}
    \]

    Then $\judgesimty E {S'} T$ by transitivity
    hence $\judgesub E {S'} T$ 
    so 
    $\judgesimt E s {\casttwoapp {S'} T t} T$
    by \rel{Up-Add}
  \end{lamproof} % CC-Chk

  \proofbreak
  
  \rulecase{C-Arrow}
  \begin{lamproof}
    In this case
    \[
    \begin{array}[t]{l@{\qquad}l}
      \judgeT E {\lamt x {S_1} {S_2}} 
      & \judgect E {\lamt x {S_1} {S_2}} {\lamt x {T_1} {T_2}}
      \\
      \judgeT E {S_1} & \judgect E {S_1} {T_1} 
      \\
      \judgeT {E,x:S_1} {S_2} & \judgect {E,x:T_1} {S_2} {T_2}
    \end{array}
    \]

    Then by induction, using narrowing:
    \[
    \begin{array}[t]{l}
      \judgesimty E {S_1} {T_1} \\
      \judgesimty {E,x:T_1} {S_2} {T_2} \\
      \judgesimty {E,x:S_1} {S_2} {T_2} \\
    \end{array}
    \]
      
    Hence by \rel{Up-Arrow} we 
    have $\judgesimty E {\lamt x {S_1} {S_2}} {\lamt x {T_1} {T_2}}$
  \end{lamproof} % C-Arrow
  
  \rulecase{C-Base}
  \begin{lamproof}
    In this case
    \[
    \begin{array}[t]{l@{\qquad}l}
      \judgeT E {\predty x B s} & \judgect E {\predty x B s} {\predty x B t}
      \\
      \judge {E,x:B} s \Bool & \judgecc {E,x:B} s t {} \Bool
    \end{array}
    \]

    Then by induction $\judgesimt {E,x:B} s t \Bool$
    and applying \rel{Eq-Base} we have 
    $\judgesimty E {\predty x B s} {\predty x B t}$ 
    \qed
  \end{lamproof} % C-Arrow
\end{lamproof} % Compilation is upcasting

%====================================================================================

\restatewtprogaccepted
\begin{lamproof} 
\pf\ By mutual induction on the typing derivation 
and well-formed type derivation.

\begin{enumerate}
\item % Part 1.
\begin{lamproof}
\rulecase{T-Var, T-Const} Immediate.

\rulecase{T-Sub} Straightforward induction

\rulecase{T-Fun}
In this case, there exists $T,t,T'$ such that
\[
\begin{array}{ll}
  \judge{E}{(\lam{x}{S}{s})}{(\lamt{x}{S}{S'})} 	&\mbox{conclusion}\\
  \judgeT{E}{S} 			&\mbox{antecedent}\\
  \judge{E,x:S}{s}{S'}		&\mbox{antecedent}\\
  \\
  \judgect{E}{S}{T}		&\mbox{induction}\\
  \judgeeq{E}{S}{T}		&\mbox{Lemma~\ref{lem:castinsertbisim}} \\
  \judge{E,x:T}{s}{S'}		&\mbox{Lemma~\ref{lemma:narrowing} (Narrowing)}\\
  \judgec{E}{s}{t}{T'}		&\mbox{induction}\\
  \judgec{E}{(\lam{x}{S}{s})}{(\lam{x}{T}{t})}{(\lamt{x}{T}{T'})}
  &\mbox{\rel{C-Fun}}
\end{array}
\]

\rulecase{T-App}
In this case, there exists $T_1,t,T,T'$ such that
\[
\begin{array}{ll}
  \judge{E}{\app{s_1}{s_2}}{S'[x:=s_2]}	&\mbox{conclusion}\\
  \judge{E}{t_1}{(\lamt{x}{S}{S'})} 	&\mbox{antecedent}\\
  \judge{E}{t_2}{S} 			&\mbox{antecedent}\\
  \\
  \judgec{E}{s_1}{t_1}{T_1}		&\mbox{induction}\\
  \judgesub{E}{T_1}{(\lamt{x}{S}{S'})} 	&\mbox{Lemma~\ref{lem:castinsertbisim}} \\
  T_1=(\lamt{x}{T}{T'}) 			&\mbox{\rel{S-Arrow}}\\
  \judgesub{E}{S}{T}			&\mbox{\rel{S-Arrow}}\\
  \judgecc{E}{s_2}{t_2}{}{T}		&\mbox{induction}\\
  \judgec{E}{\app{s_1}{s_2}}{\app{t_1}{t_2}}{T'[x:=t_2]}&\mbox{\rel{C-App}}\\
\end{array}
\]

\rulecase{T-Cast}
In this case, there exists $T_1,T_2,t$ such that
\[
\begin{array}{ll}
  \judge{E}{\castapp {S_2} s}{S_2}	&\mbox{conclusion}\\
  \judge{E}{s}{S_1}		 	&\mbox{antecedent}\\
  \judgeT{E}{S_2} 			&\mbox{antecedent}\\
  \\
  \judgeT{E}{S_1} \\
  \judgect{E}{S_1}{T_1}			&\mbox{induction}\\
  \judgect{E}{S_2}{T_2}			&\mbox{induction}\\
  \judgeeq{E}{S_1}{T_1}			&\mbox{Lemma~\ref{lem:castinsertbisim}} \\
  \judgecc{E}{s}{t}{}{T_1}			&\mbox{induction}\\
  \judgec{E}{\castapp {S_2} s}{\castapp {T_2} s}{T_2}
  &\mbox{\rel{C-Cast}}\\
\end{array}
\]

\rulecase{T-Sub} 
If $\judge{E}{s}{S}$ via \rel{T-Sub}  then $\judge{E}{s}{S'}$ for some $S'$ and this case holds by induction
\end{lamproof}

\item %Part 2.
  From $\judge{E}{s}{S}$ by induction there exists $t,U$ such that $\judgec{E}{s}{t}{U}$.
  By Lemma~\ref{lem:castinsertbisim}, $\judgesub{E}{U}{S}$, and by the transitivity of subtyping, $\judgesub{E}{U}{T}$.
  
  If $\judgesubalg{\pyes}{E}{U}{T}$ then $\judgecc{E}{s}{t}{}{T}$ via~\rel{CC-Ok}.
  
  Otherwise, by Lemma~\ref{lem:sub:sound}, $\judgesubalg{\pmaybe}{E}{U}{T}$, and hence
  $\judgecc{E}{s}{\castapp{T}t}{}{T}$ via~\rel{CC-Chk}.
  
\item %Part 3.
  \rel{WT-Arrow}, \rel{WT-Base} Straightforward induction. \qed
\end{enumerate}
\end{lamproof}

\subsection{Implication Relations}
\label{sec:implicationproofs}
Including proofs that our example implication relations satisfy the
necessary axioms.

The standard type rules for simply-typed $\lambda$-calculus terms
are:

{\footnotesize
\STLCtyperules
}

Then our translation of an implication judgement into
a formula quantifying over STLC-terms satisfies
all the properties due to properties of 
implication in higher-order logic.
\mynote{Do we even need to mention this?  For detailed proofs,
we need to chose a logic and do inductions or whatever.}

Steps:

\begin{lemma}
  If $\judge E t S$ then for all $\sigma$ consistent with $E$,
  $\sigma(t) \in \meaningf{\sigma(S)}$
\end{lemma}

\begin{lemma}
  Then $\sigma \circ \subst x t {}$ is consistent with $E,x:S$.
\end{lemma}

\begin{lemma}
  Hence subst holds
\end{lemma}
